# Supplementary material for: Atomic-Scale Origins of Oxidation Resistance in Amorphous Boron Nitride
Source: arXiv:2510.10326 ancillary file (2025-10-11)
Supplement: Supplementary file 1 [file oxidation_abn_suppmat.pdf]

# Supplementary Information: Atomic-Scale Origins of Oxidation Resistance in Amorphous Boron Nitride

Onurcan Kaya,[†,‡,¶] Qiushi Deng,[§] Thomas Souvignet,[‖] Catherine Marichy,[‖] Catherine Journet,[‖] Ivan Cole,[§] and Stephan Roche[*,†,⊥]

†*Catalan Institute of Nanoscience and Nanotechnology (ICN2), CSIC and BIST, Campus UAB, 08193 Bellaterra, Barcelona, Spain*

‡*School of Engineering, RMIT University, Melbourne, Victoria 3001, Australia*

¶*Department of Electronic Engineering, Universitat Autònoma de Barcelona (UAB), Campus UAB, 08193 Bellaterra, Barcelona, Spain*

§*School of Engineering, The Australian National University, Canberra, ACT 2600, Australia*

‖*Université Claude Bernard Lyon 1, CNRS, LMI UMR 5615, 69100 Villeurbanne, France*

⊥*ICREA, 08010 Barcelona, Spain*

E-mail: stephan.roche@icn2.cat

# Machine Learned Interatomtic Potentials

## Training Set Generation

To enable accurate and scalable molecular dynamics simulations of oxygen interaction with $\alpha$-BN, we developed a machine-learning interatomic potential within the GAP framework.[1–3]

The GAP model was trained specifically for the B–N–O system, incorporating a diverse and physically rich dataset of structures that span molecular, crystalline, and disordered phases. The dataset used to train and validate the GAP model consisted the atomic positions, energies, and forces, calculated using Car–Parrinello molecular dynamics and density functional theory (DFT) with the Quantum ESPRESSO package.[4–6] The training process followed an iterative, active learning scheme: (1) a large number of initial structures were generated by calculating the energies and forces of molecular compounds, crystalline phases, and amorphous structures containing B, N, and O atoms; (2) an initial GAP model was trained on this dataset; (3) a new set of validation structures was generated using the previously trained GAP model; (4) the energy and force predictions of the GAP model were evaluated using DFT calculations. These training–validation cycles were repeated until the lowest RMSE values were achieved. Additionally, the accuracy of the final model was further assessed by comparing structural and energetic properties, as described below.

The "training" set used to generate and validate the final GAP model contains approximately 2000 structures, while the final validation set comprises 2000 structures. Together, the dataset includes around 200000 atomic environments. A detailed breakdown by system type, number of atoms per configuration, and number of configurations is provided in Table S1. The dataset spans a wide variety of configurations to ensure comprehensive coverage of relevant atomic environments. Initially, we incorporated several molecular compounds of B,N, and O, available in the Materials Project database.[7] Crystalline forms of BN were also included using the same source. These crystalline samples were obtained from the Materials Project[7] and expanded into supercells with random strains and defects (vacancies, Stone–Walls defects, oxygen impurities) to enrich configurational diversity. To cover disordered regimes, we generated a large number of liquid and quenched structures. These include randomly generated $\alpha$-$B_xN_yO_z$ configurations, where $x$, $y$, and $z$ are random values constrained by $x + y + z = 1$. All amorphous and liquid samples contain 64 atoms per unit cell, with cubic cell geometries. Cell parameters were randomly assigned to ensure that the resulting

densities span the range 1.0-–3.5 g/cm$^3$. Periodic boundary conditions were applied to all systems. For 2D structures, a 10 Å vacuum spacing was added along the $z$-direction; for isolated atoms and molecular compounds, vacuum was added in all three spatial directions.

All configurations were labelled using *ab initio* calculations to obtain total energies and

Table S1: Breakdown of the training and validation datasets by system type, number of atoms per configuration, and total number of configurations used for GAP model development.

| **System** | **Num. of Atoms** | **Num. of ConFigure** |
|---|---|---|
| Isolated elements (B, N, O) | 1 | 3 |
| Small molecules ($B_2$, $N_2$) | 2–16 | 100 |
| Crystalline phases (e.g.,h-BN, c-BN, defected structures) | 4–64 | 1000 |
| Amorphous structures (e.g., $\alpha$-BN, $\alpha$-$B_xN_yO_z$) | 64 | 3000 |

atomic forces using Quantum ESPRESSO.[4,6] Initially, we employed Car–Parrinello MD with ultrasoft pseudopotentials (USPP) and LDA, with kinetic–energy cutoffs of 20 Ry for wavefunctions and 150 Ry for charge density, to generate and relax amorphous and liquid snapshots. Γ-point sampling was used for the Car–Parrinello MD runs on amorphous/liquid cells. The ionic timestep was 0.20 fs, the fictitious electronic mass 400 a.u., and trajectories were run for a total of 10 ps at 5000 K followed by 5 ps cool-down segments. A Nosé–Hoover thermostat in the NVT ensemble was used during Car–Parrinello MD. The crystalline and molecular structures were taken from the Materials Project;[7] the only change was adding a large vacuum.

All dataset labels were obtained from DFT calculations using PBE pseudopotentials with PAW functionals. Here, we employed a plane-wave cutoff of 75 Ry for wavefunctions and 600 Ry for charge density. When structures were relaxed, ionic steps continued until all forces were below 0.001 a.u. SCF energy convergence was $10^{-8}$ Ry. A Gaussian smearing of 0.1 eV was applied during DFT calculations. For crystalline and slab systems we used Monkhorst–Pack meshes (6×6×6 for 3D and 6×6×1 for monolayers); Γ-only was used for large amorphous/liquid cubes. Energies used for training/validation are total energies.

## Training of the GAP Model

This approach provides near-DFT accuracy while enabling simulations of tens of thousands of atoms over nanosecond timescales—regimes inaccessible to direct first-principles methods. As mentioned above, the model was trained using an iterative scheme. Starting from an initial training set, at each round we identified configurations whose forces and energies were poorly predicted by the current GAP and added those to the training set to improve the next fit. The final training set contained approximately 2000 unique configurations, with a complementary validation set comprising 2000 structures not used during training. Descriptors used in the GAP model are two-body (2b), three-body (3b), and smooth overlap of atomic positions (SOAP), with cutoffs and hyperparameters optimised to balance accuracy and efficiency, summarized in Table S2. The SOAP descriptor was sparsified using the CUR algorithm,[8] while 2b and 3b descriptors used uniform sparsification.[3] Regularization parameters for expected errors on energies and forces were set to 0.002 eV and 0.2 eV/Å, respectively. The model was trained using the QUIP package.

Table S2: Hyperparameters used to train the GAP potential for B-N-O.

| | 2-body | 3-body | SOAP |
|---|---|---|---|
| $\delta$ (eV) | 2.0 | 0.1 | 0.1 |
| $r_{cut}$ (Å) | 3.7 | 3.0 | 5.0 |
| $r_{\Delta}$ (Å) | | | 0.5 |
| $\sigma_{at}$ (Å) | | | 0.5 |
| $n_{max}$, $l_{max}$ | | | 8,8 |
| $\zeta$ | | | 4 |
| Sparsification | Uniform | Uniform | CUR |
| $N_t$ (Amorphous/liquid B-N-O) | | 150 | 3000 |
| $N_t$ (Crystalline BN, strained, defected) | | 50 | 1000 |
| $N_t$ (Total) | 25 | 200 | 4000 |

## Validation of the GAP Model

In order to assess the quality of the trained GAP for future predictions on C-doped BN samples, we compared the energies per atom and forces obtained with the GAP with the exact values from DFT calculations. Figure S1 shows that the shows the scatter plots of the mentioned values from DFT and from the GAP potentials as computed on the training and validation datasets. A significantly small value for the Root Mean Squared Error (RMSE) is found in all the training data, slightly increasing on the validation set since the latter has not been used to train the potential. The overall agreement is consequently good and no trace of overfitting is observed.

To further validate the potential, we relaxed h-BN and c-BN with both DFT and the GAP model and compared the lattice parameters. For DFT relaxations, the same PAW pseudopotentials and cutoffs used for dataset labelling were applied. The results show excellent agreement between DFT and GAP: the in-plane lattice parameter of h-BN is a=2.509 Å by DFT (PBE/PAW) and a=2.501 Å by GAP (error: 0.32%); for c-BN, $a = 3.615$ Å by DFT and $a = 3.609$ Å by GAP (error: 0.17%). These values are consistent with literature ranges. We also evaluated oxygen chemisorption on monolayer h-BN for two configurations (Figure S2): a single O on a B-N bridge (hBN:O) and two O atoms (hBN:2O). The adsorption energy is defined as

$$E_{ads}(n) = E_{hBN:nO} - E_{hBN} - \frac{n}{2} E_{O_2},$$

where $E_{hBN:nO}$ is the total energy of the chemisorbed system, $E_{hBN}$ is the energy of clean h-BN, and $E_{O_2}$ is the energy of an oxygen molecule. DFT and GAP values for the two configurations are listed in Table S3.

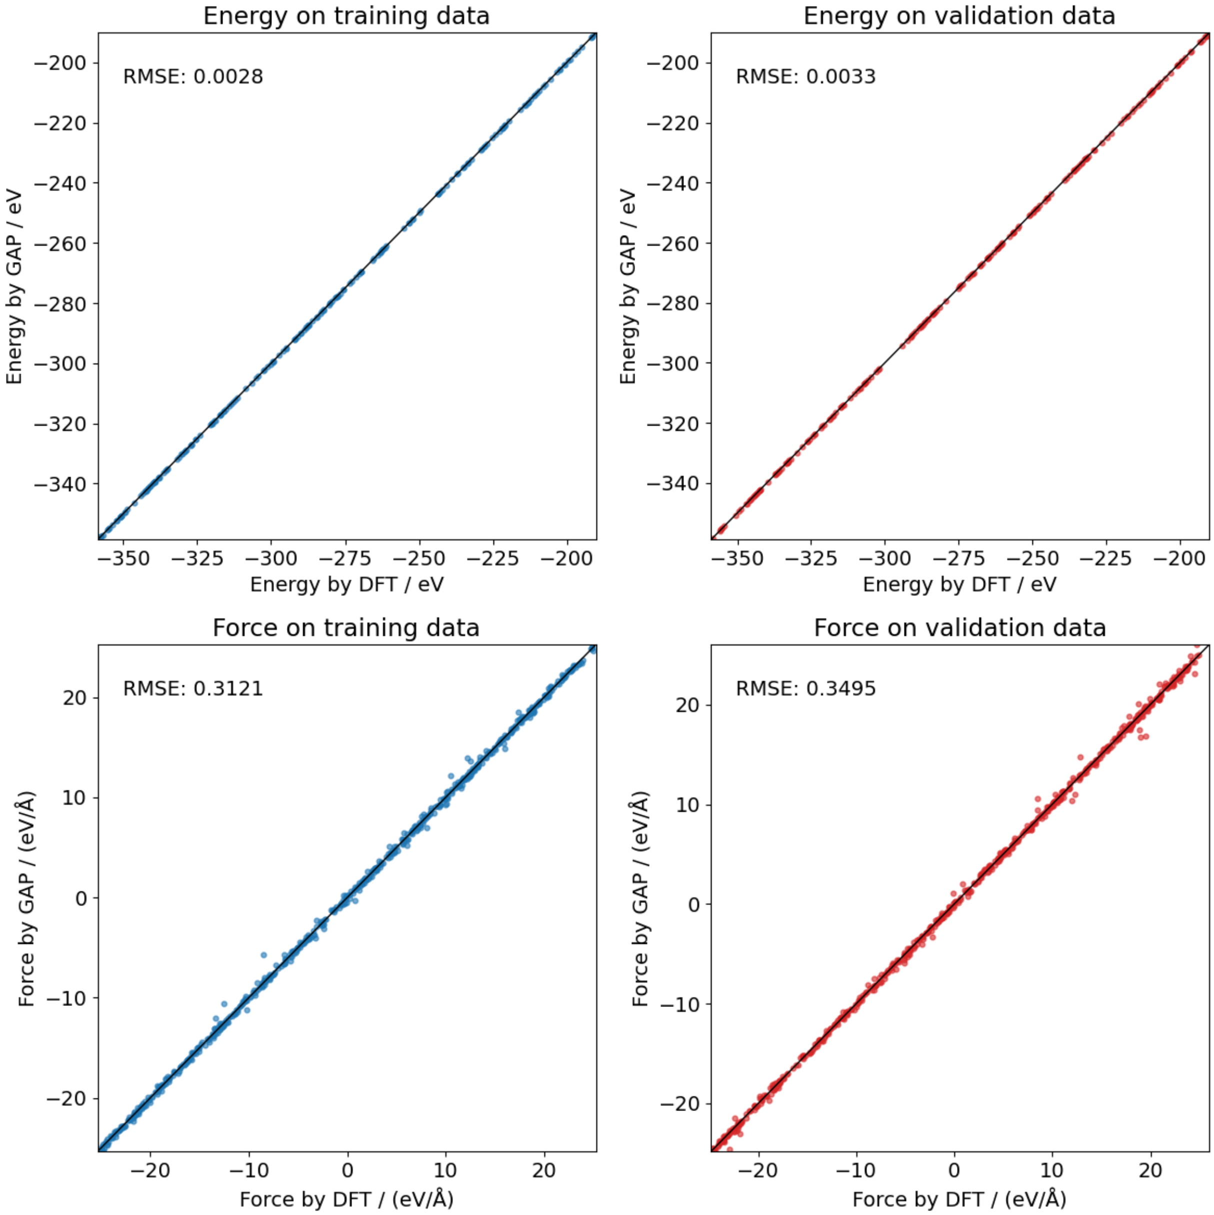


Figure S1: Scatter plots of the energies and forces obtained using GAP as a function of the corresponding DFT values. Values are computed on the training (left) and validation (right) datasets.

| Site | $E_{ads}^{DFT}$ | $E_{ads}^{GAP}$ | $\Delta$ |
|---|---|---|---|
| hBN:O | 2.13 | 2.06 | 3.29% |
| hBN:2O | 2.27 | 2.18 | 3.96% |

Table S3: O adsorption on monolayer h-BN.

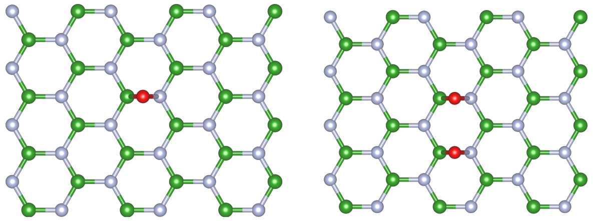

(a) hBN:O (b) hBN:2O

Figure S2: Chemisorption configurations corresponding to Table S3 where green atoms are B, gray atoms are N, and red atoms are O.

# Raman Spectra of CVD-grown Films

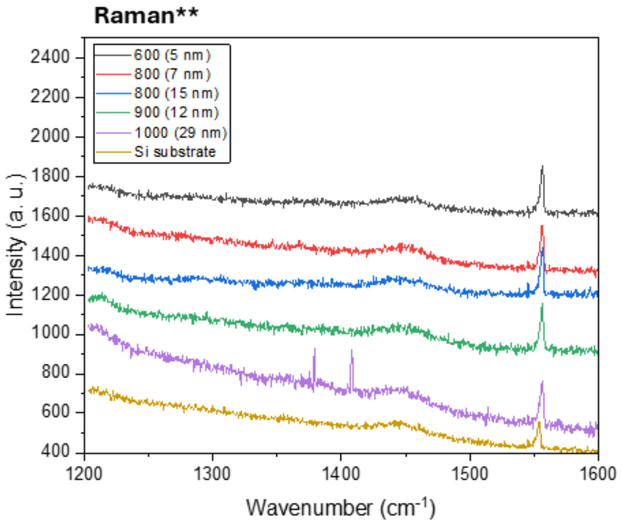


Figure S3: Raman spectra of the films used in the experimental measurements (red and green). Other films are also added for comparison.

# XPS Spectra of $\alpha$-BN Films

Table S4: Chemical composition of $\alpha$-BN films used in the study.

| Sample | O | N | C | B | Si |
|---|---|---|---|---|---|
| $\alpha$-BN-900 before exposing to air | 16.29 | 26.64 | 15.2 | 34.16 | 7.71 |
| $\alpha$-BN-800 before exposing to air | 23.4 | 17.43 | 16.6 | 26.36 | 16.21 |
| $\alpha$-BN-900 after exposing to air | 16.74 | 27.06 | 16.1 | 32.49 | 7.6 |
| $\alpha$-BN-800 after exposing to air | 24.28 | 17.64 | 15.51 | 24.63 | 17.94 |

Table S5: Angular measurements for $\alpha$-BN films.

| Sample (condition) | 90 | 50 | 35 | 27 | 20 |
|---|---|---|---|---|---|
| $\alpha$-BN-900 before exposing to air | 1.27 | 1.21 | 1.26 | 1.25 | 1.26 |
| $\alpha$-BN-900 after exposing to air | 1.29 | 1.27 | 1.27 | 1.22 | 1.25 |
| $\alpha$-BN-800 before exposing to air | 1.31 | 1.39 | 1.29 | 1.37 | 1.35 |
| $\alpha$-BN-800 before exposing to air | 1.26 | 1.34 | 1.3 | 1.27 | 1.37 |

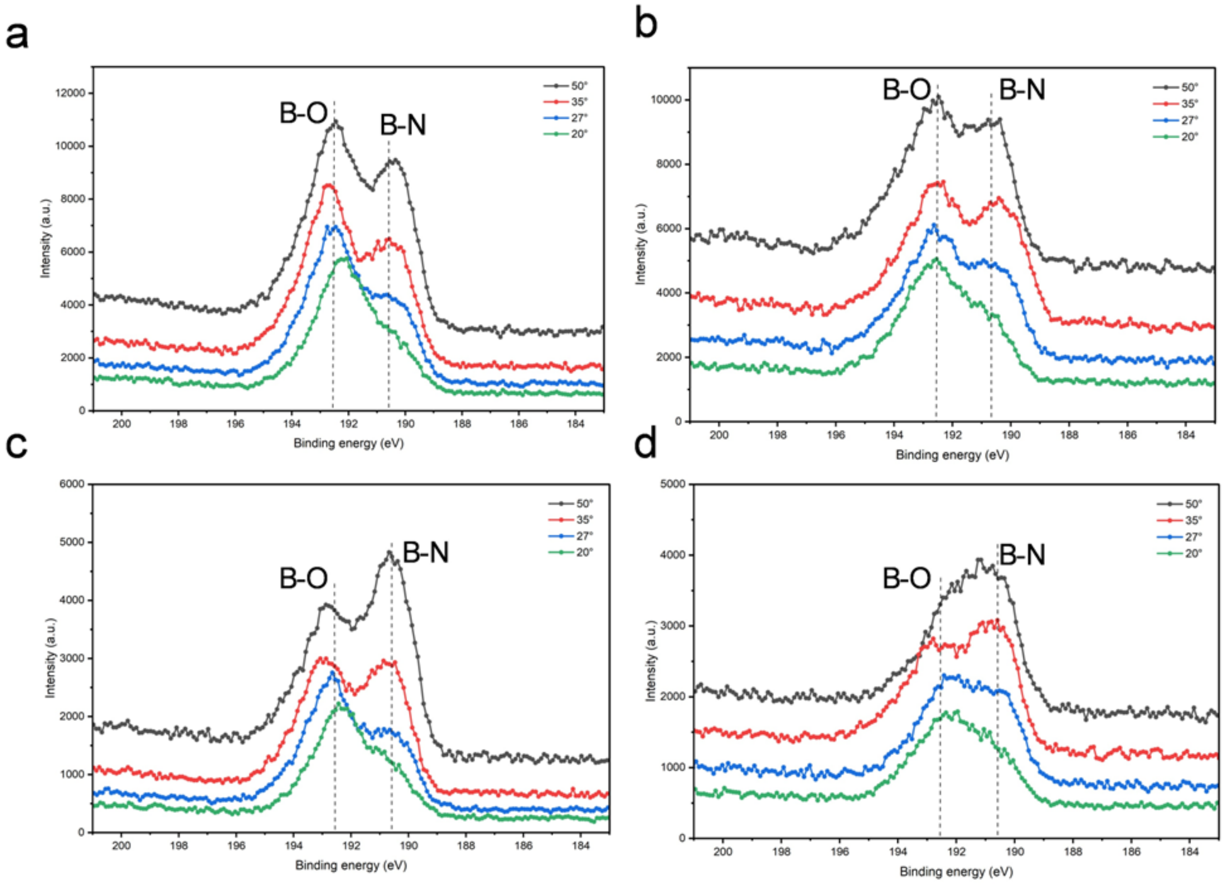


Figure S4: XPS core-level B 1s spectra of sample surface collected at different take-off angles $\alpha$-BN-900 before and after exposure(a, c); $\alpha$-BN-800 before and after exposure (b, d).

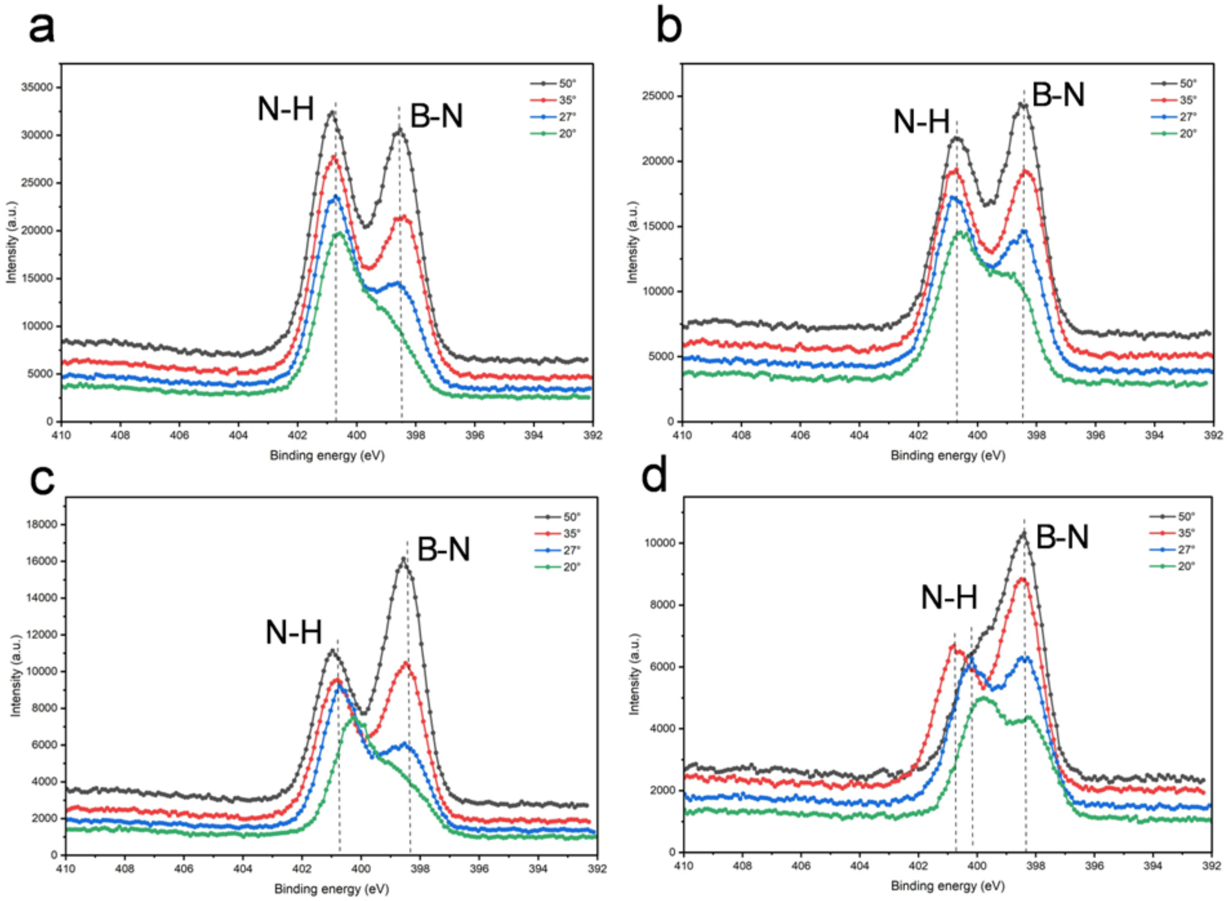


Figure S5: XPS core-level N 1s spectra of sample surface collected at different take-off angles $\alpha$-BN-900 before and after exposure (a, c); $\alpha$-BN-800 before and after exposure (b, d).

## References


1. Bartók, A. P.; Payne, M. C.; Kondor, R.; Csányi, G. Gaussian Approximation Potentials: The Accuracy of Quantum Mechanics, without the Electrons. *Physical Review Letters* **2010**, *104*, 136403.

2. Bartók, A. P.; Kondor, R.; Csányi, G. On representing chemical environments. *Phys. Rev. B* **2013**, *87*, 184115.

3. Bartók, A. P.; Csányi, G. Gaussian approximation potentials: A brief tutorial introduction. *International Journal of Quantum Chemistry* **2015**, *115*, 1051–1057.

4. Giannozzi, P.; Baroni, S.; Bonini, N.; Calandra, M.; Car, R.; Cavazzoni, C.; Ceresoli, D.; Chiarotti, G. L.; Cococcioni, M.; Dabo, I.; others QUANTUM ESPRESSO: a modular and open-source software project for quantum simulations of materials. *Journal of physics: Condensed matter* **2009**, *21*, 395502.

5. Giannozzi, P.; Andreussi, O.; Brumme, T.; Bunau, O.; Nardelli, M. B.; Calandra, M.; Car, R.; Cavazzoni, C.; Ceresoli, D.; Cococcioni, M.; others Advanced capabilities for materials modelling with Quantum ESPRESSO. *Journal of physics: Condensed matter* **2017**, *29*, 465901.

6. Giannozzi, P.; Baseggio, O.; Bonfà, P.; Brunato, D.; Car, R.; Carnimeo, I.; Cavazzoni, C.; De Gironcoli, S.; Delugas, P.; Ferrari Ruffino, F.; others Quantum ESPRESSO toward the exascale. *The Journal of Chemical Physics* **2020**, *152*, 154105.

7. Jain, A.; Ong, S. P.; Hautier, G.; Chen, W.; Richards, W. D.; Dacek, S.; Cholia, S.; Gunter, D.; Skinner, D.; Ceder, G.; Persson, K. A. Commentary: The Materials Project: A materials genome approach to accelerating materials innovation. *APL Materials* **2013**, *1*, 011002.

8. Mahoney, M. W.; Drineas, P. CUR matrix decompositions for improved data analysis. *Proceedings of the National Academy of Sciences* **2009**, *106*, 697–702.
